# Supplementary material for: Direct-PoseNet: Absolute Pose Regression with Photometric Consistency
Source: arXiv:2104.04073 source file (2021-10-13)
Supplement: Supplementary file 1 [file algo1.tex]

\begin{algorithm}[!t]
   \SetAlgoLined
   \SetKwInOut{Input}{Input}
   \SetKwInOut{Output}{Output}
   \Input{Image $I$, Pose regression model $\mathcal{G}_\Psi$,\\NeRF model $\mathcal{F}_\Theta$.}
   
   \Output{Optimized pose regression model $\mathcal{G}_{\Psi^*}$.}
   
   \KwData{Train set $\mathcal{D}_t$ and Validation set $\mathcal{D}_v$.}
   
   \BlankLine
   Initialize $\mathcal{G}$ with pre-trained weight $\Psi$\;
   $loss_{min} = \infty$; $c = 0$;~\tcp{early stopping counter}
   \While{$c < patience$}{
      \ForEach {batch $b \in \mathcal{D}_t$}{
         $loss_{train} = \mathcal{L}(I, \lambda_1, \lambda_2, \mathcal{G}_\Psi, \mathcal{F}_\Theta)$\;
         %// update the model weights\;
        %  ${\Psi^*} \leftarrow \Psi - \beta \nabla_{\Psi} \mathcal{L}(\mathcal{G}_\Psi)$\;
        ${\Psi^*} \leftarrow \text{backpropagate}(loss_{train})$\;
         $\Psi = \Psi^*$\;
      }

      \ForEach{batch $b \in \mathcal{D}_v$}{
         $loss_{val} = \mathcal{L}_{gt}(I, \mathcal{G}_{\Psi^*})$\;
      }
      \eIf{$loss_{val} < loss_{min}$}{
         $loss_{min} = loss_{val}$\;
         $c=0$\;
      }{
         $c=c + 1$\;
      }
  }
   \Return{$\mathcal{G}_{\Psi^*}$}%return $G_\phi$
   \caption{Train pose regression model with direct matching}
   \label{algo:1}
\end{algorithm}
